# Supplementary material for: Two-sided fairness in rankings via Lorenz dominance
Source: arXiv:2110.15781 source file (2021-10-28)
Supplement: Supplementary file 2 [file leximin_utilitarian.tex]

\section{Leximin order}

\subsection{One-sided recommendation}

The most egalitarian trade-off achievable by our method is described by the leximin order \citep{sen1979equality}. Given two utility profiles $\bu$ and $\bv$,  $\bu\leximinw\bv$ if $\bucum$ is greater than $\bvcum$ according to the lexicographic order.\footnote{Formally, $\bu\leximin\bv$ if $(\exists k\in\intint{d}$ s.t. $\forall i< k$, $\bucum_i=\bvcum_i$ and $\bucum_k>\bvcum_k)$. ~~$\bu\leximinw\bv \iff \lnot(\bv\leximinw\bu)$.} The leximin optimal profile is egalitarian in the sense that it maximizes the utility of individuals in sequence, from the worse-off to the better-off. Depending on the set of feasible profiles, this may not lead to equal utility for everyone, but any further reduction of inequality can only be achieved by making people worse off for the benefit of no other, in violation of Pareto-dominance.

%First, we show that if $\alpha_1$ and $\alpha_2$ both converge to infinity at a comparable rate $\alpha$, i.e., $\alpha_1 = \alpha\eta_1$ and $\alpha_2=\alpha\eta_2$ for $\eta_1, \eta_2>0$, then the optimal utility profile is leximin optimal over both users and items, where $\eta_1$ and $\eta_2$ control how user and item utilities are compared with each other. Second, 
In Appendix~\ref{sec:leximin}, we show that item-side leximin-optimal rankings are found by keeping $\alpha_1$ constant and having $\alpha_2\to-\infty$, in cases where $\lambda$ converges to $1$ faster than $\alpha_2$ tends to $-\infty$ .
On the other end of achievable trade-offs lies the utilitarian ranking ($\alpha_1=\alpha_2=1)$, which we analyze below. 

\begin{restatable}{proposition}{proputilitarian1sided} \label{prop:utilitarian-1sided}
Let $\rrkopt\in\argmaxPl \W_{\frac{1}{2}, 1, 1}(\rrk) = \argmaxPl \sumUls \tuiP + \sumIls \tujP$ be the \emph{utilitarian ranking}. Then $\forall \bv\in\US, {\tu}_{\userS}(\rrkopt)\leximinw\bvusers$.
\end{restatable}
The utilitarian ranking is also the leximin optimal on the user side. Any attempt to reduce inequality in user utilities can only decrease the utility of some users for the benefit of no other. This shows that fundamentally, the concept of user-side fairness (defined as driving towards more equity in user utility) is of practical significance only in a context of two-sided fairness. In that case, preference for equity on the user side means that transfers between users and items mostly comes at the expense the most satisfied users.

\subsection{Reciprocal recommendation}

\paragraph{Utilitarian ranking} Proposition~\ref{prop:utilitarian} below generalizes to two-sided utilities the well-known result that maximizing user-side utility $\UiP$ is achieved by sorting $j\in\itemS$ by decreasing $\muij$ (see e.g., \citep{cossock2008statistical}). The proof is in Appendix \ref{sec:proofswelfare}. For a ranking tensor $\rrk$ and a user $i$, we denote by $\rkS(\rrki)$ the support of $\rrki$ in ranking space.%
\footnote{Formally, $\rkS(\rrki)=\xSet[\big]{\sigma:\itemS\rightarrow\intint{\nitems}\big | \,\sigma \text{~is one-to-one, and~}\forall j\in\itemS, \rrk_{ij\sigma(j)} > 0}$.} 
We remind that $\sigma(j)$ is the rank of item $j$, and that lower ranks are better.
\begin{restatable}[Utilitarian ranking]{proposition}{proputilitarian} \label{prop:utilitarian}
Let $\rrkopt\in\argmaxPls \W_{\frac{1}{2}, 1, 1}(\rrk) = \argmaxPls \sum\limits_{i\in\intint{\n}} \tuiP$.
%be the \emph{utilitarian ranking}. Then, $\forall i\in\userS$:
%for every ranking $\sigma_i$ in the support of $\rrkopt_i$, we have: $\sigma_i(j) < \sigma_i(j') \implies \tmuij \geq \tmuijprime$.
\begin{enumerate}[leftmargin=*]
    \item $\displaystyle \forall i\in\userS, \forall \sigma\in\rkS(\rrkopti):
    \sigma(j) < \sigma(j') \implies \tmuij \geq \tmuijprime
    \text{~~with~~} \tmuij=\muij+\muji.$
    \item If $\forall (i,j)\in\intint{n}^2, \muij=\muji$, then $\tmuij\geq \tmuijprime\iff \muij\geq\mu_{ij'}$.
\end{enumerate}
\end{restatable}
When mutual preferences are symmetric, the utilitarian ranking is the same as the usual sort by decreasing $\muij$. This means that without considerations of two-sided fairness ($\alpha_1, \alpha_2<1$), the optimal ranking for two-sided utilities is the same as the usual ranking. This might explain why the two-sided utility has never been studied before, even in reciprocal recommendation \citep{palomares2021reciprocal}.
